# Supplementary material for: Thermal Magnetic Fluctuations of a Ferroelectric Quantum Critical Point
Source: arXiv:2009.12995 ancillary file (2020-09-28)
Supplement: Supplementary file 1 [file Supplemental.pdf]

# Supplemental material for " Thermal Magnetic Fluctuations of a Ferroelectric Quantum Critical Point "

Alexander Khaetskii[1], Vladimir Juričić[2], and Alexander V. Balatsky[1,2]

[1]*Department of Physics, University of Connecticut, Storrs, CT 06269, USA*

[2]*Nordita, KTH Royal Institute of Technology and Stockholm University, Roslagstullsbacken 23, SE-106 91 Stockholm, Sweden*

## I. DERIVATION OF THE EXPRESSION FOR THE MAGNETIC SUSCEPTIBILITY WITHIN THE KUBO FORMALISM

We start by evaluating the following commutator for the magnetization, which is given in terms of the polarization field by Eq. (1) in the main text,

$$[M_i(t), M_j(0)] = \epsilon_{ikl}\epsilon_{jmn}\lambda^2\{P_k(t)\frac{\partial P_l(t)}{\partial t}P_m(0)\frac{\partial P_n(0)}{\partial t} - P_m(0)\frac{\partial P_n(0)}{\partial t}P_k(t)\frac{\partial P_l(t)}{\partial t}\}.$$

Using the Wick's theorem, we obtain for the average

$$\langle[M_i(t), M_j(0)]\rangle = (8/9)\lambda^2\delta_{ij}\{\langle P(t)P(0)\rangle\langle\dot{P}(t)\dot{P}(0)\rangle + \langle P(0)\dot{P}(t)\rangle\langle\dot{P}(0)P(t)\rangle$$
$$- \langle P(0)P(t)\rangle\langle\dot{P}(0)\dot{P}(t)\rangle - \langle P(t)\dot{P}(0)\rangle\langle\dot{P}(t)P(0)\rangle\}, \quad \text{(S1)}$$

where the correlators of the polarization field are

$$\langle P(t)P(0)\rangle = \gamma^2\frac{1}{V}\sum_{\mathbf{q}} A_q^2[e^{i\mathbf{qr}-i\omega_\perp t}(1+N_q) + e^{-i\mathbf{qr}+i\omega_\perp t}N_q],$$
$$\langle\dot{P}(t)\dot{P}(0)\rangle = \gamma^2\frac{1}{V}\sum_{\mathbf{q}} A_q^2[e^{i\mathbf{qr}-i\omega_\perp t}(1+N_q) + e^{-i\mathbf{qr}+i\omega_\perp t}N_q]\omega_\perp^2(q),$$
$$\langle P(0)\dot{P}(t)\rangle = \gamma^2\frac{1}{V}\sum_{\mathbf{q}} A_q^2[-i\omega_\perp e^{i\mathbf{qr}-i\omega_\perp t}N_q + i\omega_\perp e^{-i\mathbf{qr}+i\omega_\perp t}(N_q+1)]. \quad \text{(S2)}$$

The remaining correlators are found from the symmetry relations

$$\langle P(0)P(t)\rangle = \langle P(t)P(0)\rangle^\star,\ \langle\dot{P}(0)\dot{P}(t)\rangle = \langle\dot{P}(t)\dot{P}(0)\rangle^\star,$$
$$\langle\dot{P}(0)P(t)\rangle = -\langle P(0)\dot{P}(t)\rangle,\ \langle P(t)\dot{P}(0)\rangle = \langle\dot{P}(0)P(t)\rangle^\star,$$
$$\langle\dot{P}(t)P(0)\rangle = \langle P(0)\dot{P}(t)\rangle^\star.$$

While deriving the above expressions we used that $\langle\hat{b}_{\xi,\mathbf{q}}\hat{b}^\dagger_{\xi_1,\mathbf{q}_1}\rangle = \delta_{\xi,\xi_1}\delta_{\mathbf{qq}_1}(N_q+1)$, $\langle\hat{b}^\dagger_{\xi,\mathbf{q}}\hat{b}_{\xi_1\mathbf{q}_1}\rangle = \delta_{\xi,\xi_1}\delta_{\mathbf{qq}_1}N_q$, where $N_q = N_B(\omega_\perp(q))$ is the Bose distribution function. Moreover, since the transverse phonon excitations are softer than the longitudinal optical ones, we neglected the latter, i.e. $\omega_\xi = \omega_\perp$. We also use the following relation

$$\sum_{\mathbf{q}}...\sum_{\xi=\pm}\overline{h^i_{\xi,\mathbf{q}}h^j_{\xi,\mathbf{q}}} = \sum_{\mathbf{q}}...(\delta_{ij} - e^i_{\mathbf{q}}\,e^j_{\mathbf{q}}) \approx \sum_{\mathbf{q}}...(1-\langle(e^i_{\mathbf{q}})^2\rangle)\delta_{ij} = \sum_{\mathbf{q}}...(2/3)\delta_{ij}.$$

Here the summation over $\xi = \pm$ accounts for the two polarizations of the transverse phonon, $\mathbf{e_q} = \mathbf{q}/q$ is a unit vector in the direction of the vector $\mathbf{q}$, and the bar means averaging over the orientations of the vector $\mathbf{h}$ in the plane perpendicular to $\mathbf{q}$.

Using the expressions for the correlators presented above, we obtain for the thermally averaged commutator

$$\langle [M_i(\mathbf{r},t), M_j(0)] \rangle = \delta_{ij} \frac{i\hbar\Lambda}{V^2} \sum_{\mathbf{q},\mathbf{q}_1} N_q \sin[\mathbf{q}_1\mathbf{r} - \mathbf{q}\mathbf{r} + \omega_\perp(q)t - \omega_\perp(q_1)t], \tag{S3}$$

where $\Lambda = (16/9)\lambda^2\gamma^4\hbar(a_0^3/\bar{M}_0)^2$. Using now Eq. (S3) we obtain the form of the susceptibility presented in the main text.

## II. DERIVATION OF EQ. (7) IN THE MAIN TEXT

In this Section, we derive Eq. (7) starting with Eq. (6) in the main text. As a first step, for small $k \ll q$ we expand the quantity $\omega_\perp(q) - \omega_\perp(|\mathbf{q} - \mathbf{k}|)$. At $T \ll \hbar\omega_0$ (the case we consider here), the characteristic $q$ satisfies the inequality $s_0 q \ll \omega_0$. Then the above mentioned expansion acquires the form $\omega_\perp(q) - \omega_\perp(|\mathbf{q} - \mathbf{k}|) = (s_0^2/2\omega_0)(2\mathbf{k}\mathbf{q} - k^2)$. Thus from Eq. (6) we find

$$\begin{aligned}
\chi(\omega,\mathbf{k}) &= -\Lambda \int \frac{d^3q}{(2\pi)^3} \frac{N[\omega_\perp(q)]}{\omega + i0 + (s_0^2/2\omega_0)(2kqx - k^2)} + \big\{\omega + i0 \to -\omega - i0\big\} \\
&= -\Lambda \int_0^\infty \frac{q^2 dq}{(2\pi)^2} N(\omega_\perp(q)) \frac{\omega_0}{s_0^2 kq} J.
\end{aligned} \tag{S4}$$

Here $x = \mathbf{k}\cdot\mathbf{q}/kq$, and

$$J = \int_{-1}^{+1} dx \; \frac{1}{[(\omega + i0)\omega_0/s_0^2 kq] - (k/2q) + x} + \big\{\omega + i0 \to -\omega - i0\big\}.$$

Integration over $x$ can be straightforwardly performed and yields

$$J = \ln \frac{(1 - k/2q)^2 - A^2}{(1 + k/2q)^2 - A^2} \approx -\left(\frac{2k}{q}\right) \frac{1}{1 - A^2},$$

where we used the expansion for $k/q \ll 1$, and $A = (\omega + i0)\omega_0/s_0^2 kq$. Substituting the above expression for $J$ into Eq. (S4), we obtain Eq. (7) of the main text.
